# Supplementary material for: Erratum: Photovoltage from ferroelectric domain walls in BiFeO$_3$
Source: arXiv:1905.10321 source file (2025-03-06)
Supplement: Supplementary file 1 [file article_and_suppmat.pdf]

# Photovoltage from ferroelectric domain walls in BiFeO<sub>3</sub>

Sabine Körbel and Stefano Sanvito

*School of Physics, AMBER and CRANN Institute, Trinity College, Dublin 2, Ireland\**

We calculate the component of the photovoltage in bismuth ferrite that is generated by ferroelectric domain walls, using first-principles methods, in order to compare its magnitude to the experimentally measured photovoltage. We find that excitons at the ferroelectric domain walls form an electric dipole layer resulting in a domain-wall driven photovoltage. This is of the same order of magnitude as the experimentally measured one, but only if the carrier lifetimes and diffusion lengths are larger than previously assumed.

Keywords: Condensed Matter & Materials Physics, Ferroelectric Domains, First-principles calculations, DFT+U, Photovoltaic Effect, Exciton, Perovskite

**Introduction** It has long been debated if and to what extent ferroelectric domain walls contribute to the photovoltaic effect (PVE) in ferroelectric oxides like BaTiO<sub>3</sub> and BiFeO<sub>3</sub>. One possible origin of the PVE in BiFeO<sub>3</sub> is the so-called bulk photovoltaic effect (BPVE) [1–6]. The BPVE is a phenomenological term describing any photovoltaic effect that takes place in the homogeneous interior of the material, as opposed to interface effects. The BPVE in ferroelectrics such as BiFeO<sub>3</sub> and BaTiO<sub>3</sub> has been ascribed to noncentrosymmetric scattering or relaxation of electrons and holes after photoexcitation in noncentrosymmetric crystals, resulting in a net shift of charge carriers (“shift current”) [2, 3, 5, 6]. The BPVE depends on the polarization direction of the incoming light [4]. This dependence was indeed observed in the case of BiFeO<sub>3</sub>, and it was hence concluded that the BPVE is at the origin of the photovoltaic effect in BiFeO<sub>3</sub> [7, 8].

Alternatively a domain-wall driven PVE (DW-PVE) has been proposed [9–11]. The argument in favor of the DW-PVE is a variation in the ferroelectric polarization of the atomic lattice at the domain walls. It has been suggested that this polarization variation gives rise to internal electrostatic fields at the domain walls. If true, this would mean that ferroelectric domain walls could separate photogenerated charge carriers in the same way as *p-n* junctions, without the need for *p*- and *n*-type doping, and it would be possible to align arbitrarily many such junctions in series and add up the individual voltages created by each single junction. However, the DW-PVE theory needs to postulate a local ferroelectric polarization not only of the spatially discrete atomic lattice, but also for the continuum of the valence electrons. But is it possible to define and determine the electric polarization of an arbitrary section of a crystal? Only then can this local polarization induce an electric field. Such approach was adopted in previous first-principles studies of voltage steps/drops at ferroelectric domain walls in PbTiO<sub>3</sub> [12] and BiFeO<sub>3</sub> [9] and yielded electrostatic potential drops (electronic potential steps) ranging from 0.02 to 0.2 V per domain wall for the dark state (without illumination). We will demonstrate below that this polarization-based approach does not yield the correct sign of the potential step/drop and the photoinduced charge density at domain walls in BiFeO<sub>3</sub>. In contrast to the BPVE, the DW-PVE is independent of the polarization direction of the incoming light.

Some studies [6, 13] take the middle ground by assuming

that the BPVE and the DW-PVE may exist simultaneously and can be cooperative or antagonistic depending on the system geometry. The argumentation here is that, besides the characteristic angular dependence of the BPVE with respect to the polarization of the incoming light, there is a polarization-independent offset in the photocurrent, which might be ascribed to a DW-PVE originating in an electrostatic field at the ferroelectric domain walls [6], and/or in a locally modified BPVE, caused by the local crystal-structure modifications at the domain walls [13].

Whereas the atomistic structure of ferroelectric domain walls in BiFeO<sub>3</sub> is accurately known thanks to electron microscopy [14], experimental spectroscopy of photoelectrons at ferroelectric domain walls with atomic resolution is to our knowledge not possible today, but is perfectly within reach of first-principles calculations based on density-functional theory (DFT). In fact, optical excitations and the spatial distributions of the photoexcited charge carriers in molecules and solids are nowadays routinely investigated by means of many-body perturbation theory [15–18], such as the Bethe-Salpeter equation, or time-dependent density-functional theory. In the case of ferroelectric domain walls such studies would be hard to undertake because of the large system size needed to model a domain wall. However, there are approximate methods with a favorable balance between accuracy and computational cost, such as the excitonic  $\Delta$ -self-consistent-field ( $\Delta$ SCF) method, which yields more than qualitative agreement with highly accurate many-body methods [19], but can be performed at the same computational cost as a DFT ground-state calculation. The excitonic  $\Delta$ SCF approach has been applied to study excitons in various systems, including organic dyes [20], polymers [19, 21], and surfaces [22]. Here we use it to directly determine the magnitude of the domain-wall driven photovoltaic effect in BiFeO<sub>3</sub>, as given by the electronic potential induced by excitons localized at the domain walls.

**Methods** We focus on the 71° and the 109° domain wall, for which the direction of the ferroelectric polarization in adjacent domains differs by about 71° and by 109°, respectively. In rhombohedral perovskites like BiFeO<sub>3</sub> there exists also a 180° domain wall; however, due to its symmetry it should be photovoltaically inactive, and hence we do not consider it here. The DFT calculations were performed with the VASP code [24], using the projector-augmented wave (PAW)

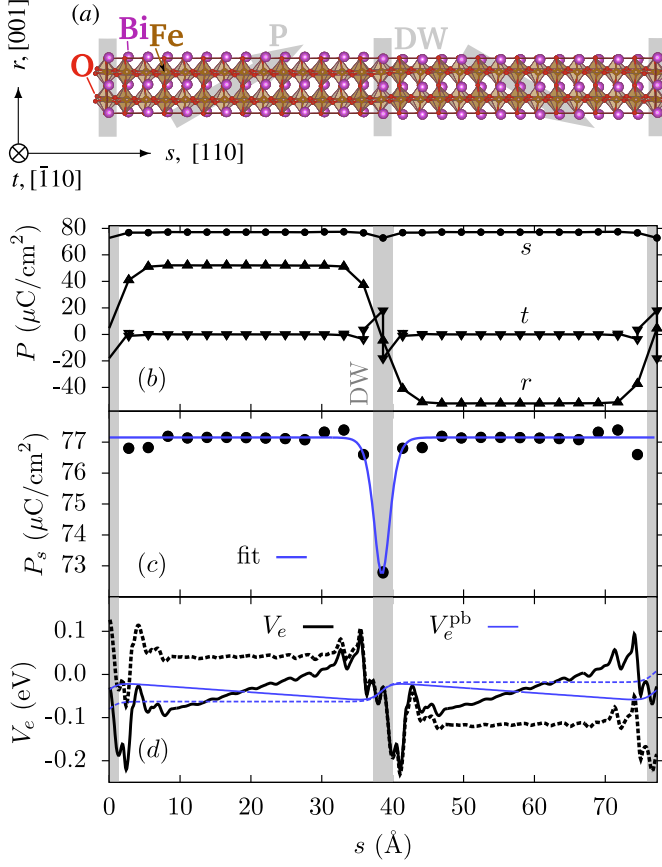

FIG. 1. (Color online) 71° domain wall: (a) 280-atom supercell with two domain walls, (b) all three components of the ferroelectric polarization  $P$ , (c) polarization component  $P_s$  perpendicular to the domain wall, and (d) polarization-based electronic potential energy  $V_e^{\text{pb}}$  and electronic potential energy  $V_e$  directly obtained from DFT (thick black lines), shifted to zero and smoothened [23]. The dashed lines in (d) denote open-circuit conditions.

method and pseudopotentials with 5 (Bi), 16 (Fe), and 6 (O) valence electrons, respectively. We employed the local-spin-density approximation, and corrected the  $3d$  states of Fe with a Hubbard- $U$  of 5.3 eV following Dudarev’s scheme [25]. The  $U$  value for Fe was taken from the “materials project” database [26] and it is optimized for oxide formation energies, but it also yields an optical band gap of 2.54 eV close to the experimental one of  $\approx 2.7$ –2.8 eV [27–32]. This computational setup yields structural properties of BiFeO<sub>3</sub> in reasonable agreement with experiment [23, 33–37]. The reciprocal space was sampled with  $2 \times 5 \times 3$   $k$ -points for the 71° wall and with  $2 \times 5 \times 5$   $k$ -points for the 109° wall. Plane-wave basis functions with energies up to 520 eV were used. We employed a supercell approach with periodic boundary conditions, such that each supercell contained 120–280 atoms and two domain walls. Both the atomic positions and cell parameters were allowed to relax until the energy difference between subsequent ionic relaxation steps fell below 0.1 meV. Our calculated structural properties of the domain walls are similar to

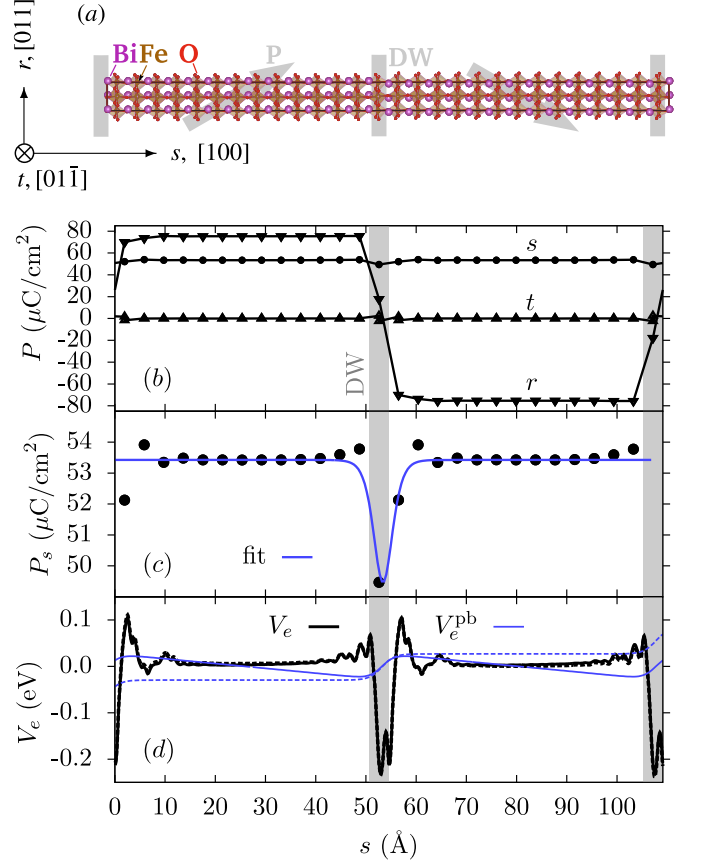

FIG. 2. (Color online) The same as Fig. 1 for the 109° domain wall.

those in previous theoretical [14, 38–40] as well as experimental [14] works [23]. Excitons were modeled with the excitonic  $\Delta\text{SCF}$  method [20], namely by occupying the valence states with altogether  $(N - N_X)$  electrons and the conduction states with  $N_X$  electrons, where  $N$  and  $N_X$  are the total number of electrons and excitons in the supercell, respectively. This was done in every iteration step of the electronic self-consistency cycle, using the same density functional for minimizing the energy as in a ground-state calculation. The geometries of the systems in the presence of an exciton were optimized when considering excitonic polaron states. Supercells containing 120 atoms were used in this case. The excitonic  $\Delta\text{SCF}$  method is suitable for exploring low-lying excited states only, whereas access to higher-lying excited states such as Rydberg states can be obtained using constrained DFT [41] or by maximizing the similarity of the excited-state orbitals to reference orbitals [42, 43]. In order to obtain the photovoltage per domain wall,  $V_{\text{photo}}^{\text{DW}}$ , we first determine the photovoltage profile,  $V_{\text{photo}}$ , which is given by the difference in electronic potential between the excited state,  $V_e^X$ , and the ground state,  $V_e^{\text{GS}}$ :

$$V_{\text{photo}}(s) = [V_e^X(s) - V_e^{\text{GS}}(s)] / (-|e|), \quad (1)$$

where  $s$  is the coordinate perpendicular to the domain wall. The domain-wall contribution  $V_{\text{photo}}^{\text{DW}}$  is then equal to the amplitude of the spatial variation of the photovoltage profile at

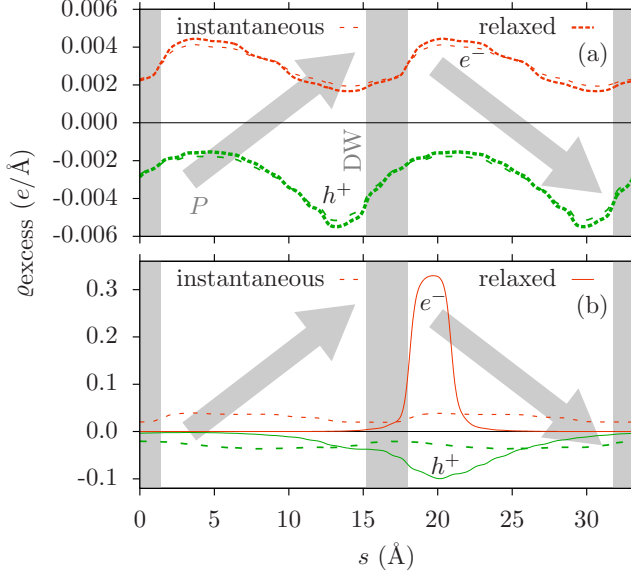

FIG. 3. (Color online) Smoothed densities of excess electrons and holes for excitons (X) at the 71° domain wall before (“instantaneous”) and after (“relaxed”) polaron formation: (a) for an X density of 0.1 X per 120-atom supercell (a planar X density of  $\approx 2.3 \times 10^{13}$  X/cm²) a large polaron forms, (b) for an X density of 1 X per 120-atom supercell ( $\approx 2.3 \times 10^{14}$  X/cm²) a small polaron forms. Gray bars and arrows indicate ferroelectric domains.

the domain wall (compare Fig. 6),

$$V_{\text{photo}}^{\text{DW}} = V_{\text{photo}}(s_{\text{DW}}^-) - V_{\text{photo}}(s_{\text{DW}}^+), \quad (2)$$

where  $s_{\text{DW}}^{\pm}$  are positions to the right and to the left of the domain wall. We calculate both  $V_e^X$  and  $V_e^{\text{GS}}$  in the ground-state structure. By doing so, the electronic screening is already included. We still need to consider the screening by the lattice, which we calculate *ab initio* [23]. Note that, since we are working with DFT,  $V_e$  is the Kohn-Sham potential. Furthermore, the use of periodic boundary conditions implies that we are calculating the short-circuit potential. The open-circuit potential is then obtained from the short-circuit potential by adding a constant gradient that compensates the potential slope in the domain interior [12]. The photovoltages are extrapolated [23, 44] to avoid finite-size effects.

**Results and discussion** We begin the discussion with the electronic potential at the ferroelectric domain walls in the ground state (without excitons). Figure 1 depicts the ferroelectric polarization, the electronic potential energy per electron,  $V_e$ , and the polarization-based potential energy per electron,  $V_e^{\text{pb}}$ , as calculated from the polarization variation at the wall including screening [23]. If the polarization-based approach was valid,  $V_e^{\text{pb}}$  should yield the same potential step/drop at the wall as  $V_e$ .  $V_e$  has a potential minimum on the right-hand side of the wall. Accordingly, we expect excess electrons to accumulate on the right-hand side of the wall. The magnitude of the electronic potential drop (the electrostatic potential step) at the wall is 0.13 eV (extrapolated [23]).

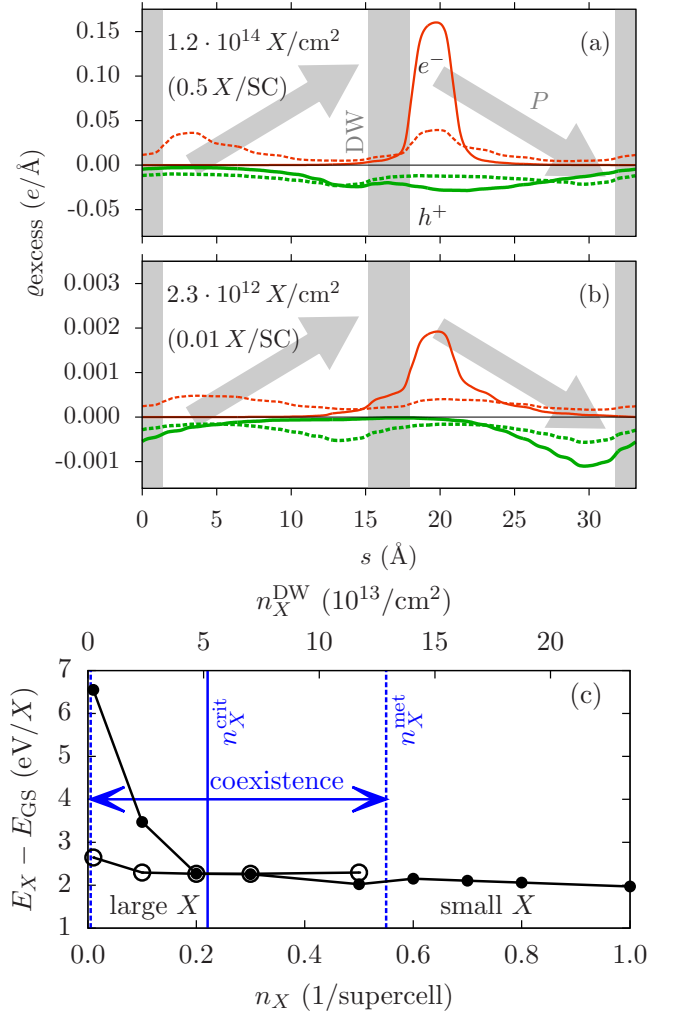

FIG. 4. (Color online) Smoothed densities of excess electrons and holes for exciton (X) densities in the coexistence region of the large (dashed line) and the small (solid line) X polaron in a 120-atom supercell (SC) with 71° domain walls. (a) For a planar X density  $n_X^{\text{DW}}$  of  $\approx 1.2 \times 10^{14}$  X/cm² the small X polaron is stable and the large X polaron is metastable. (b) For a planar X density of  $\approx 2.3 \times 10^{12}$  X/cm² the large X polaron is stable and the small X polaron is metastable. (c) Formation energies of the small (small filled circles) and the large (large empty circles) X polaron. The large X polaron is stable for X densities below  $n_X^{\text{crit}}$  and between  $n_X^{\text{crit}}$  and  $n_X^{\text{met}}$  it is metastable.

$V_e^{\text{pb}}$  exhibits an electronic potential step at the wall instead of a potential drop, and the magnitude of the potential variation, 45 meV, is too small. For the 109° domain wall (Fig. 2) the potential has a pronounced minimum inside the domain wall, and a very small slope in the domain interior corresponding to an electronic potential drop of about 17 meV [23].  $V_e^{\text{pb}}$  lacks the minimum inside the wall, and exhibits an electronic potential step instead of a potential drop, and the magnitude of the potential variation, 56 meV, is too large. We conclude that the polarization-based approach fails to provide the correct sign and magnitude of potential steps/drops at domain walls in BiFeO<sub>3</sub>.

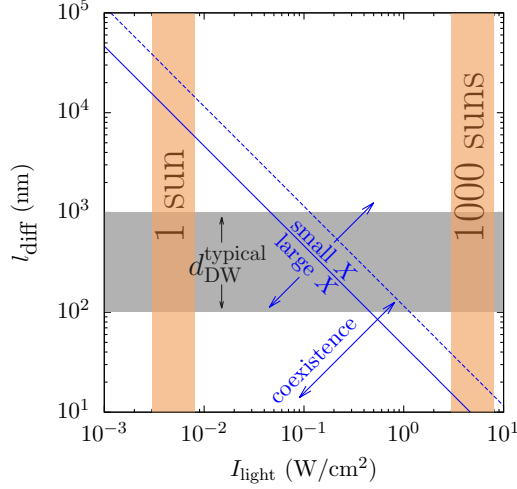

FIG. 5. (Color online) Excitonic phase diagram. The solid blue line indicates the critical light intensity as a function of the carrier diffusion length  $l_{\text{diff}}$  according to Eq. (6) in the Supplemental Material; the dashed blue line marks the upper boundary of the coexistence region of the small and the large exciton polarons. Orange vertical bars mark the intensity of sunlight and thousandfold concentrated sunlight above the band gap of BiFeO<sub>3</sub>, and the gray horizontal bar marks a range of typical domain-wall spacings  $d_{\text{DW}}$  found in the experimental literature.

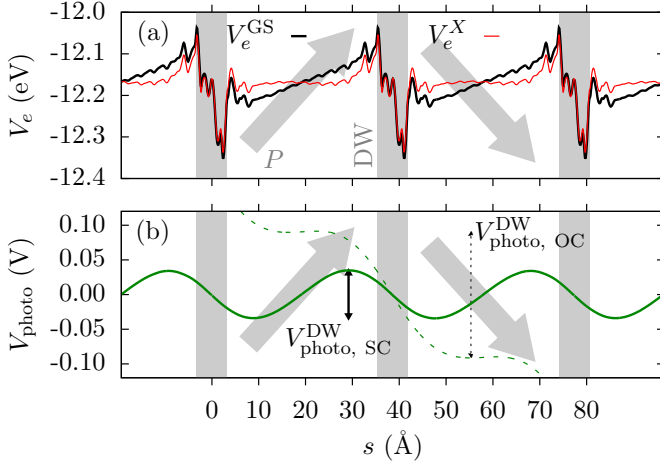

FIG. 6. (Color online) (a) Smoothed potential energy of electrons at the 71° domain wall in the ground state ( $V_e^{\text{GS}}$ ) and in the excited state ( $V_e^{\text{X}}$ ) in a 280-atom supercell with 0.1 excitons. (b) Instantaneous photovoltage profile  $V_{\text{photo}}$  [cf. Eq. (1)] for short-circuit (solid line) and open-circuit conditions (dashed line). Green arrows show the magnitude of the domain-wall photovoltage  $V_{\text{photo}}^{\text{DW}}$ .

Next, we will add an electron-hole pair (an exciton) to our supercell. Depending on the exciton density, two different types of exciton polarons form, as depicted in Fig. 3. For low exciton densities, a large exciton forms with photoelectrons and -holes localized on opposite sides of the domain wall resulting in an excitonic dipole moment. Note that the sign of

the photoinduced charge density (electron on the right-hand side of the wall, hole on the left) is the same as one would expect based on the electronic potential drop (the electrostatic potential step) in the ground state, but it is opposite to what one would expect based on the polarization-based potential (electron on the left-hand side of the wall, hole on the right). The same is true for individual electrons and holes [45]. At high exciton densities a small, almost concentric exciton polaron forms (a self-trapped exciton) with a negligible dipole moment. Figure 4 shows the densities of excess electrons and holes for different densities of exciton polarons in the 120-atom supercell, and the excitation energy per exciton of the large and the small exciton polaron. There is a critical exciton density above which the large exciton polaron transforms into a small exciton polaron (above which the formation energy of the small exciton polaron becomes lower than that of the large exciton polaron), and a coexistence region in which either the large or the small exciton polaron is stable and the other one is metastable. Since only the large exciton configuration will lead to a sizable photovoltage, we determine next under which experimental conditions the large exciton forms.

In Ref. 46 it was found that the photocurrent in BiFeO<sub>3</sub> follows a rate equation,  $\dot{n} = g - n/\tau$ , where  $n$  is the photocarrier density,  $g$  is the photocarrier generation rate, and  $\tau \approx 75 \mu\text{s}$  is the photocarrier lifetime. Here we adopt the same rate equation for the exciton density  $n_X$ , which in the steady state is given by

$$n_X = g\tau = \frac{I_{\text{light}}(1-R)\tau}{E_{\text{photon}}d_{\text{film}}}, \quad (3)$$

where  $I_{\text{light}}$  is the intensity of the light in W/cm<sup>2</sup>,  $d_{\text{film}}=100$  nm is the thickness of the experimentally studied films in Refs. 7 and 11,  $E_{\text{photon}}=3.06$  eV is the photon energy of the laser used in the experiment in Ref. 7, and  $R \approx 0.27$  is the reflectivity calculated at this photon energy from first principles. In the following we assume that 100% of the penetrating light is absorbed [23], in line with experiment [47]. We assume further that all photocarriers within a distance  $l_{\text{diff}}$  (the diffusion length) from the domain wall reach the domain wall. Figure 4(b) shows that the critical exciton density from the supercell calculation is  $n_X^{\text{crit}} \approx 0.22 X$  per supercell, corresponding to an planar exciton density of  $\approx 5.2 \times 10^{13}/\text{cm}^2$ . This is equal to a photoelectron density of  $3.7 \times 10^{18}/\text{cm}^3$  if one assumes a diffusion length of 140 nm. From Eq. (3) we obtain the critical light intensity for the transition between large and small exciton polarons [23], which is depicted in Fig. 5. In the case of natural sunlight and a diffusion length near typical domain-wall spacings of a few hundred nanometers, the large exciton forms, which should give rise to a photovoltage, whereas in the case of a thousandfold concentrated sunlight, such as in a concentrator solar-cell setup, the small exciton polaron forms, which should contribute less to the photovoltage, if at all. The small exciton polaron might be detectable with photoluminescence spectroscopy as a state inside the band gap, or as a drop in the photovoltage at illumination intensities of

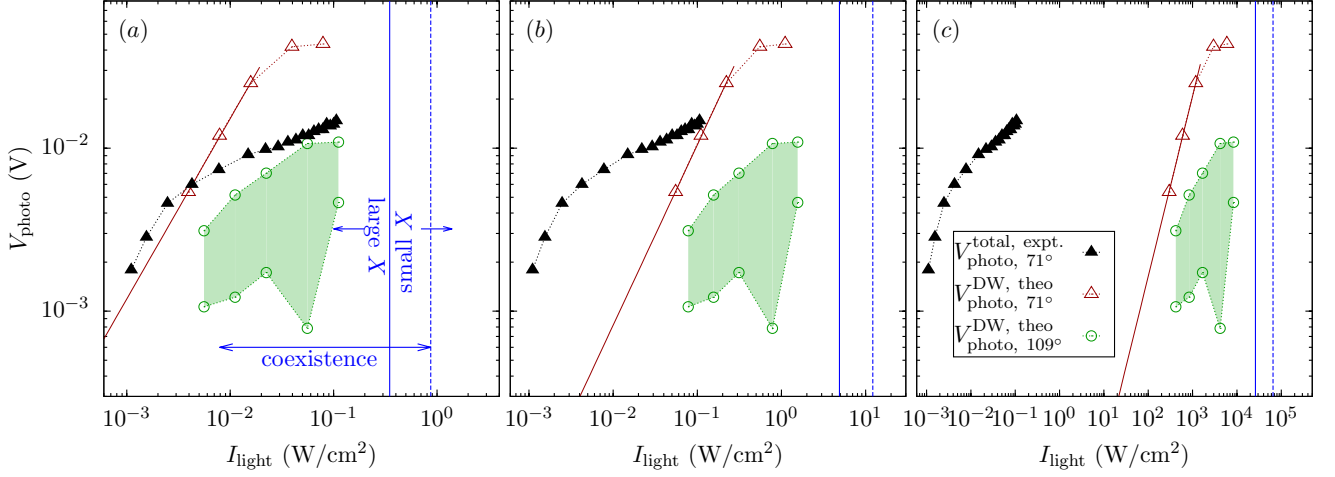

FIG. 7. (Color online) Measured photovoltage per domain of BiFeO<sub>3</sub> films with 71° domain walls from Ref. 11 and calculated domain-wall photovoltage of the 71° and the 109° domain walls as a function of the illumination intensity for different photocarrier life times  $\tau$  and diffusion lengths  $l_{\text{diff}}$ : (a)  $\tau = 75 \mu\text{s}$ ,  $l_{\text{diff}} = 140 \text{ nm}$ ; (b)  $\tau = 75 \mu\text{s}$ ,  $l_{\text{diff}} = 10 \text{ nm}$ ; (c)  $\tau = 1 \text{ ns}$ ,  $l_{\text{diff}} = 140 \text{ nm}$ . Solid lines are an extrapolation; dotted lines are a guide to the eye.

the order of 0.1–1 W/cm<sup>2</sup> or higher, depending on the carrier diffusion length.

In the following we consider moderate light intensities, at which the large exciton forms. The domain-wall photovoltage is the spatial potential variation induced by the large exciton at the domain wall, depicted in Fig. 6. The potential generated by the excitons (partially) compensates the electronic potential drop (the electrostatic potential step) at the domain wall. The relation between exciton density and light intensity is the same as before, now we use the parameters of the experimental photovoltage measurement from Ref. 11 in Eq. (3) ( $E_{\text{photon}} = 3.31 \text{ eV}$ ,  $R = 0.25$ , domain-wall spacing  $d_{\text{DW}} = 140 \text{ nm}$ ). These parameters are similar to those used above to determine the critical exciton density of the phase transition. As an upper limit we consider a diffusion length equal to the domain-wall spacing,  $l_{\text{diff}} = d_{\text{DW}} = 140 \text{ nm}$  [23]. We also consider an estimated lower limit of  $l_{\text{diff}} = 10 \text{ nm}$  similar to that assumed in Ref. 11, and a shorter carrier lifetime of 1 ns, similar to that reported in Ref. 48. The resulting open-circuit photovoltage contribution per domain wall, together with the experimental results from Ref. 11, are depicted in Fig. 7 and extrapolated to lower light intensities using a power law [23]. In the case of the 109° domain wall we can only give a possible range (shaded area) [23]. The experimental photovoltage is the total photovoltage of a film with 71° domain walls, consisting of all photovoltaic effects (bulk and domain-wall effects), divided by the number of domains. The experimental conditions are well inside the range in which the large exciton forms (marked by the vertical solid line), for which our approach should be valid. The calculated domain-wall photovoltage matches the experimentally measured one only in the most optimistic scenario [Fig. 7(a)], in which we assume a photocarrier density of  $10^{16}/\text{cm}^3$  to  $10^{18}/\text{cm}^3$ , a carrier lifetime of 75  $\mu\text{s}$ , and a carrier diffusion length of 140 nm.

For comparison, in Ref. 11 a carrier density of about  $10^{12}/\text{cm}^3$  to  $10^{13}/\text{cm}^3$ , a carrier diffusion length of 8 nm, and a lifetime of 35 ps were assumed, and in Ref. 48 a lifetime of 1 ns. If we assume such conditions [Figs. 7(b) and 7(c)], the DW-PVE is orders of magnitude too small to account for the major part of the measured photovoltage in BiFeO<sub>3</sub>. The domain-wall photovoltage may be further reduced through screening by free charge carriers and/or point defects that accumulate at the domain walls.

**Conclusion** We have analyzed the contribution of ferroelectric domain walls to the photovoltage in BiFeO<sub>3</sub> using first principles methods. In general we find that the ferroelectric polarization profile does not allow one to determine the correct sign and magnitude of the electrostatic potential at the domain walls. Instead the electronic potential should be directly determined from *ab initio* calculations. The domain-wall driven photovoltages can be as large as the experimentally measured total photovoltages (up to  $\approx 10 \text{ mV}$  per domain wall), and may therefore be responsible for a large portion of the photovoltaic effect in BiFeO<sub>3</sub>. This, however, is true only if the carrier lifetimes and carrier diffusion lengths are of the order of  $\approx 100 \mu\text{s}$  and  $\approx 100 \text{ nm}$ , respectively, which is orders of magnitude larger than previously assumed. Otherwise, the domain-wall photovoltage is orders of magnitude smaller, and then the major fraction of the photovoltage should originate from other effects, for example bulk effects. Furthermore, there is a transition from a large to a small exciton polaron at high illumination intensities of the order of 0.1–1 W/cm<sup>2</sup> or higher, which might be experimentally detected as a drop in the photovoltage at high light intensities, or as a state inside the band gap in photoluminescence spectroscopy.



## ACKNOWLEDGEMENT

This project has received funding from the European Union's Horizon 2020 research and innovation programme under the Marie Skłodowska-Curie Grant Agreement No. 746964. Computation time and support provided by the Trinity Centre for High Performance Computing funded by Science Foundation Ireland is gratefully acknowledged. We also thank the Irish Centre for High-End Computing (ICHEC) for the provision of computational facilities and support. We are grateful to Subhayan Roychoudhury (Trinity College Dublin) for sharing his knowledge of excited-state density-functional theory. Graphics were made using `GNU PLOT` and `VESTA` [49].

---

\* skoerbel@uni-muenster.de

- [1] V. M. Fridkin and B. N. Popov, "Anomalous photovoltaic effect in ferroelectrics," *Sov. Phys. Usp.* **21**, 981 (1978).
- [2] Wolfgang Kraut and Ralph von Baltz, "Anomalous bulk photovoltaic effect in ferroelectrics: a quadratic response theory," *Phys. Rev. B* **19**, 1548 (1979).
- [3] Ralph von Baltz and Wolfgang Kraut, "Theory of the bulk photovoltaic effect in pure crystals," *Phys. Rev. B* **23**, 5590 (1981).
- [4] V.M. Fridkin, "Bulk photovoltaic effect in noncentrosymmetric crystals," *Crystallogr. Rep.* **46**, 654–658 (2001).
- [5] Steve M. Young and Andrew M. Rappe, "First Principles Calculation of the Shift Current Photovoltaic Effect in Ferroelectrics," *Phys. Rev. Lett.* **109**, 116601 (2012).
- [6] Steve M Young, Fan Zheng, and Andrew M Rappe, "First-principles calculation of the bulk photovoltaic effect in bismuth ferrite," *Phys. Rev. Lett.* **109**, 236601 (2012).
- [7] Akash Bhatnagar, Ayan Roy Chaudhuri, Young Heon Kim, Dietrich Hesse, and Marin Alexe, "Role of domain walls in the abnormal photovoltaic effect in BiFeO<sub>3</sub>," *Nature communications* **4** (2013).
- [8] Ming-Min Yang, Akash Bhatnagar, Zheng-Dong Luo, and Marin Alexe, "Enhancement of local photovoltaic current at ferroelectric domain walls in BiFeO<sub>3</sub>," *Sci. Rep.* **7**, 43070 (2017).
- [9] Jan Seidel, Lane W Martin, Q He, Q Zhan, Y-H Chu, A Rother, ME Hawkrige, P Maksymovych, P Yu, M Gajek, *et al.*, "Conduction at domain walls in oxide multiferroics," *Nat. Mater.* **8**, 229–234 (2009).
- [10] S. Y. Yang, J. Seidel, S. J. Byrnes, P. Shafer, C.-H. Yang, M. D. Rossell, Y.-H. Chu P. Yu, J. F. Scott, J. W. Ager III, L. W. Martin, and R. Ramesh, "Above-bandgap voltages from ferroelectric photovoltaic devices," *Nat. Nanotechnol.* **5**, 143–147 (2010).
- [11] Jan Seidel, Deyi Fu, Seung-Yeul Yang, Esther Alarcón-Lladó, Junqiao Wu, Ramamoorthy Ramesh, and Joel W Ager III, "Efficient photovoltaic current generation at ferroelectric domain walls," *Phys. Rev. Lett.* **107**, 126805 (2011).
- [12] B Meyer and David Vanderbilt, "Ab initio study of ferroelectric domain walls in PbTiO<sub>3</sub>," *Phys. Rev. B* **65**, 104111 (2002).
- [13] Ryotaro Inoue, Shotaro Ishikawa, Ryota Imura, Yuuki Kitahara, Takeshi Oguchi, Yuji Noguchi, and Masaru Miyayama, "Giant photovoltaic effect of ferroelectric domain walls in perovskite single crystals," *Scientific Reports* **5**, 14741 (2015).
- [14] Yi Wang, Chris Nelson, Alexander Melville, Benjamin Winchester, Shunli Shang, Zi-Kui Liu, Darrell G Schlom, Xiaoping Pan, and Long-Qing Chen, "BiFeO<sub>3</sub> domain wall energies and structures: a combined experimental and density functional theory+U study," *Phys. Rev. Lett.* **110**, 267601 (2013).
- [15] Xavier Blase, Ivan Duchemin, and Denis Jacquemin, "The Bethe–Salpeter equation in chemistry: relations with TD-DFT, applications and challenges," *Chem. Soc. Rev.* **47**, 1022–1043 (2018).
- [16] Catalin D Spataru, Sohrab Ismail-Beigi, Lorin X Benedict, and Steven G Louie, "Excitonic effects and optical spectra of single-walled carbon nanotubes," *Phys. Rev. Lett.* **92**, 077402 (2004).
- [17] Pierluigi Cudazzo, Lorenzo Sponza, Christine Giorgetti, Lucia Reining, Francesco Sottile, and Matteo Gatti, "Exciton band structure in two-dimensional materials," *Phys. Rev. Lett.* **116**, 066803 (2016).
- [18] C Rödl, F Fuchs, J Furthmüller, and F Bechstedt, "Ab initio theory of excitons and optical properties for spin-polarized systems: Application to antiferromagnetic MnO," *Phys. Rev. B* **77**, 184408 (2008).
- [19] Emilio Artacho, M Rohlfing, M Côté, P. D. Haynes, R. J. Needs, and C Molteni, "Structural Relaxations in Electronically Excited Poly(para-phenylene)," *Phys. Rev. Lett.* **93**, 116401 (2004).
- [20] Tim Kowalczyk, Shane R Yost, and Troy Van Voorhis, "Assessment of the  $\Delta$ SCF density functional theory approach for electronic excitations in organic dyes," *J. Chem. Phys.* **134**, 054128 (2011).
- [21] Davide Ceresoli, Erio Tosatti, Sandro Scandolo, G Santoro, and S Serra, "Trapping of excitons at chemical defects in polyethylene," *J. Chem. Phys.* **121**, 6478–6484 (2004).
- [22] Oleg Pankratov and Matthias Scheffler, "Localized excitons and breaking of chemical bonds at III-V (110) surfaces," *Phys. Rev. Lett.* **75**, 701 (1995).
- [23] See Supplemental Material at <http://link.aps.org/supplemental/10.1103/PhysRevB.102.081304> for figures and tables with calculation results for crystal structure, domain-wall properties, and photovoltage, compared with the literature where available, and technical details. .
- [24] Georg Kresse and Jürgen Furthmüller, "Efficiency of ab-initio total energy calculations for metals and semiconductors using a plane-wave basis set," *Comput. Mater. Sci.* **6**, 15–50 (1996).
- [25] S. L. Dudarev, G. A. Botton, S. Y. Savrasov, C. J. Humphreys, and A. P. Sutton, "Electron-energy-loss spectra and the structural stability of nickel oxide: An LSDA+U study," *Phys. Rev. B* **57**, 1505–1509 (1998).
- [26] Anubhav Jain, Shyue Ping Ong, Geoffroy Hautier, Wei Chen, William Davidson Richards, Stephen Dacek, Shreyas Cholia, Dan Gunter, David Skinner, Gerbrand Ceder, and Kristin A. Persson, "The Materials Project: A materials genome approach to accelerating materials innovation," *APL Materials* **1**, 011002 (2013).
- [27] S. R. Basu, L. W. Martin, Y. H. Chu, M. Gajek, R. Ramesh, R. C. Rai, X. Xu, , and J. L. Musfeldt, "Photoconductivity in BiFeO<sub>3</sub> thin films," *Appl. Phys. Lett.* **92**, 091905 (2008).
- [28] A. J. Hauser, J. Zhang, L. Mier, R. A. Ricciardo, P. M. Woodward, T. L. Gustafson, L. J. Brillson, and F. Y. Yang, "Characterization of electronic structure and defect states of thin epitaxial BiFeO<sub>3</sub> films by UV-visible absorption and cathodoluminescence spectroscopies," *Appl. Phys. Lett.* **92**, 222901 (2008).
- [29] JF Ihlefeld, NJ Podraza, ZK Liu, RC Rai, X Xu, T Heeg, YB Chen, J Li, RW Collins, JL Musfeldt, *et al.*, "Optical band gap of BiFeO<sub>3</sub> grown by molecular-beam epitaxy," *Appl. Phys. Lett.* **92**, 142908 (2008).
- [30] Amit Kumar, Ram C Rai, Nikolas J Podraza, Sava Denev, Mariola Ramirez, Ying-Hao Chu, Lane W Martin, Jon Ihlefeld,

- T Heeg, J Schubert, *et al.*, “Linear and nonlinear optical properties of BiFeO<sub>3</sub>,” *Appl. Phys. Lett.* **92**, 121915 (2008).
- [31] V Železný, D Chvostová, L Pajasová, I Vrejoiu, and M Alexe, “Optical properties of epitaxial BiFeO<sub>3</sub> thin films,” *Applied Physics A* **100**, 1217–1220 (2010).
- [32] Daniel Sando, Cécile Carrétéro, Mathieu N Grisolia, Agnès Barthélémy, Valanoor Nagarajan, and Manuel Bibes, “Revisiting the Optical Band Gap in Epitaxial BiFeO<sub>3</sub> Thin Films,” *Advanced Optical Materials* **6**, 1700836 (2018).
- [33] J. M. Moreau, C. Michel, R. Gerson, and W. J. James, “Ferroelectric BiFeO<sub>3</sub> X-ray and neutron diffraction study,” *Journal of Physics and Chemistry of Solids* **32**, 1315 – 1320 (1971).
- [34] Andrzej Palewicz, R Przeniosło, Izabela Sosnowska, and AW Hewat, “Atomic displacements in BiFeO<sub>3</sub> as a function of temperature: neutron diffraction study,” *Acta Crystallographica Section B: Structural Science* **63**, 537–544 (2007).
- [35] A Palewicz, I Sosnowska, R Przeniosło, and AW Hewat, “BiFeO<sub>3</sub> crystal structure at low temperatures,” *Acta Physica Polonica-Series A General Physics* **117**, 296 (2010).
- [36] P Fischer, M Polomska, I Sosnowska, and M Szymanski, “Temperature dependence of the crystal and magnetic structures of BiFeO<sub>3</sub>,” *Journal of Physics C: Solid State Physics* **13**, 1931 (1980).
- [37] Delphine Lebeugle, Dorothée Colson, A Forget, and Michel Viret, “Very large spontaneous electric polarization in BiFeO<sub>3</sub> single crystals at room temperature and its evolution under cycling fields,” *Appl. Phys. Lett.* **91**, 022907 (2007).
- [38] Oswaldo Diéguez, Pablo Aguado-Puente, Javier Junquera, and Jorge Íñiguez, “Domain walls in a perovskite oxide with two primary structural order parameters: First-principles study of BiFeO<sub>3</sub>,” *Phys. Rev. B* **87**, 024102 (2013).
- [39] Yun-Wen Chen, Jer-Lai Kuo, and Khian-Hooi Chew, “Polar ordering and structural distortion in electronic domain-wall properties of BiFeO<sub>3</sub>,” *J. Appl. Phys.* **122**, 075103 (2017).
- [40] Wei Ren, Yurong Yang, Oswaldo Diéguez, Jorge Íñiguez, Narayani Choudhury, and L. Bellaiche, “Ferroelectric Domains in Multiferroic BiFeO<sub>3</sub> Films under Epitaxial Strains,” *Phys. Rev. Lett.* **110**, 187601 (2013).
- [41] Pablo Ramos and Michele Pavanello, “Low-lying excited states by constrained DFT,” *J. Chem. Phys.* **148**, 144103 (2018).
- [42] Chiao-Lun Cheng, Qin Wu, and Troy Van Voorhis, “Rydberg energies using excited state density functional theory,” *J. Chem. Phys.* **129**, 124112 (2008).
- [43] Andrew TB Gilbert, Nicholas A Besley, and Peter MW Gill, “Self-consistent field calculations of excited states using the maximum overlap method (MOM),” *J. Phys. Chem. A* **112**, 13164–13171 (2008).
- [44] Wolfgang P. Schleich, *Quantum Optics in Phase Space, Appendix E* (WILEY-VCH Verlag Berlin GmbH, 2001).
- [45] Sabine Körbel, Jirka Hlinka, and Stefano Sanvito, “Electron trapping by neutral pristine ferroelectric domain walls in BiFeO<sub>3</sub>,” *Phys. Rev. B* **98**, 100104(R) (2018).
- [46] Marin Alexe, “Local mapping of generation and recombination lifetime in BiFeO<sub>3</sub> single crystals by scanning probe photoinduced transient spectroscopy,” *Nano Lett.* **12**, 2193–2198 (2012).
- [47] Marin Alexe and Dietrich Hesse, “Tip-enhanced photovoltaic effects in bismuth ferrite,” *Nature Communications* **2**, 256 (2011).
- [48] YM Sheu, SA Trugman, Y-S Park, S Lee, HT Yi, S-W Cheong, QX Jia, AJ Taylor, and RP Prasankumar, “Ultrafast carrier dynamics and radiative recombination in multiferroic BiFeO<sub>3</sub>,” *Appl. Phys. Lett.* **100**, 242904 (2012).
- [49] Koichi Momma and Fujio Izumi, “VESTA3 for three-dimensional visualization of crystal, volumetric and morphology data,” *J. Appl. Crystallogr.* **44**, 1272–1276 (2011).

# Photovoltage from ferroelectric domain walls in BiFeO<sub>3</sub>: Supplemental Material

Sabine Körbel and Stefano Sanvito  
School of Physics, AMBER and CRANN Institute, Trinity College, Dublin 2, Ireland\*

## Calculated ground-state properties of BiFeO<sub>3</sub>

|                       | Expt                                                                                                                                                             | ideal<br>perovskite            | this work         |
|-----------------------|------------------------------------------------------------------------------------------------------------------------------------------------------------------|--------------------------------|-------------------|
| $a$ (Å)               | 5.57330(5) <sup>d</sup> ; 5.57882(5) <sup>b</sup> ;<br>5.5876(3) <sup>a</sup> ; 5.58132(5) <sup>c</sup> ;                                                        |                                | 5.5006<br>(-1.3%) |
| $c$ (Å)               | 13.84238(16) <sup>d</sup> ; 13.867(1) <sup>a</sup> ;<br>13.86932(16) <sup>b</sup> ; 13.87698(15) <sup>c</sup> ;                                                  |                                | 13.507<br>(-2.4%) |
| $c/a$                 | 2.4817 <sup>a</sup> ; 2.48370 <sup>d</sup> ;<br>2.48607 <sup>b</sup> ; 2.48633 <sup>c</sup>                                                                      | $\sqrt{6}$<br>$\approx 2.4495$ | 2.4556<br>(-81%)  |
| $V$ (Å <sup>3</sup> ) | 372.36 <sup>d</sup> ; 373.06 <sup>f</sup> ; 373.83 <sup>b</sup> ;<br>374.37 <sup>c</sup> ; 374.94 <sup>a</sup> ; 375.05 <sup>e</sup>                             |                                | 342.75<br>(-8%)   |
| $z_{\text{Fe}}$       | 0.22021(09) <sup>b</sup> ; 0.22046(8) <sup>d</sup> ;<br>0.22067(8) <sup>c</sup> ; 0.2209(5) <sup>e</sup> ;<br>0.2209(6) <sup>f</sup> ; 0.2212(15) <sup>a</sup> ; | 0.25                           | 0.227<br>(-20%)   |
| $x_{\text{O}}$        | 0.443(2) <sup>a</sup> ; 0.44506(22) <sup>d</sup> ;<br>0.4453(8) <sup>f</sup> ; 0.44582(22) <sup>c</sup> ;<br>0.4460(8) <sup>e</sup> ; 0.44694(28) <sup>b</sup>   | 0.5                            | 0.436<br>(+12%)   |
| $y_{\text{O}}$        | 0.012(4) <sup>a</sup> ; 0.01700(28) <sup>c</sup> ;<br>0.0173(12) <sup>e</sup> ; 0.01789(28) <sup>d</sup> ;<br>0.01814(35) <sup>b</sup> ; 0.0185(13) <sup>f</sup> | 0.0                            | 0.018<br>(±0%)    |
| $z_{\text{O}}$        | 0.9511(5) <sup>f</sup> ; 0.9513(5) <sup>e</sup> ;<br>0.95152(11) <sup>d</sup> ; 0.95183(14) <sup>b</sup> ;<br>0.95183(11) <sup>c</sup> ; 0.9543(20) <sup>a</sup> | 0.0                            | 0.961<br>(-15%)   |
| $\alpha$ (°)          | 59.34 <sup>c</sup> ; 59.35 <sup>b</sup> ; 59.35 <sup>e</sup> ;<br>59.39 <sup>d</sup> ; 59.39 <sup>f</sup> ; 59.42 <sup>a</sup>                                   | 60                             | 59.89<br>(-81%)   |
| $\omega$ (°)          | 12.2 <sup>c</sup> ; 12.3 <sup>b</sup> ; 12.4 <sup>c</sup> ;<br>12.5 <sup>a</sup> ; 12.5 <sup>f</sup> ; 12.6 <sup>d</sup>                                         | 0                              | 14.4<br>(+14%)    |
| $P$                   | $\approx 100^g$ ;                                                                                                                                                |                                | 94                |

<sup>a</sup> Moreau *et al.* [1]. Single crystal X-Ray and neutron powder diffraction at room temperature.

<sup>b</sup> Palewicz *et al.* [2]. Neutron powder diffraction at 298 K.

<sup>c</sup> Palewicz *et al.* [3]. Neutron powder diffraction at 298 K.

<sup>d</sup> Palewicz *et al.* [3]. Neutron powder diffraction at 5 K.

<sup>e</sup> Fischer *et al.* [4]. Neutron powder diffraction at 293 K.

<sup>f</sup> Fischer *et al.* [4]. Neutron powder diffraction at 4.2 K.

<sup>g</sup> Lebeugle *et al.* [5]. Single crystals,  $R3c$  phase, room temperature.

TABLE I. Measured (ordered by size) and calculated structure parameters of BiFeO<sub>3</sub> in the  $R3c$  phase: Hexagonal lattice constants  $a$  and  $c$ ,  $c/a$  ratio, cell volume  $V$ , fractional atomic coordinates, rhombohedral cell angle  $\alpha$ , octahedral rotation angle  $\omega$ , and ferroelectric polarization  $P$ . Errors (in brackets) are with respect to the closest experimental value. Errors of atomic coordinates,  $\alpha$ , and  $c/a$  are those of ferroelectric distortions from the ideal perovskite structure.

Table I contains our calculated structural parameters of BiFeO<sub>3</sub> in the  $R3c$  phase in comparison with experimental data. Lattice parameters deviate from experiment by about

2%, typical for LDA calculations. Ferroelectric displacements of atoms from the ideal perovskite structure deviate by up to 20%. Ferroelectric distortions of the unit cell ( $c/a$  ratio and rhombohedral cell angle) are severely underestimated by  $\approx 80\%$ , nevertheless the ferroelectric polarization is in good agreement with experiment, indicating that ferroelectric properties are well captured by our computational setup.

## Calculated domain-wall properties

In Table II we compare our calculated DW formation energies and widths for different supercell sizes with those available in the literature. For historical reasons, we include the 180° wall, although we do not consider it in the main article. Note that Ref. 6 found close agreement between domain-wall structures seen in electron microscopy and those calculated from first principles. This is true in particular for the domain-wall widths, which are as narrow as about one atomic layer in the case of the 109° domain wall and two atomic layers in the case of the 180° domain wall, both according to experiment and to first-principles calculations (see Fig. 1 and 2 in Ref. 6). The 71° domain wall is slightly broader and extends over about three atomic planes. We fitted the polarization and tilt profiles  $P$  and  $A$  with a tangens hyperbolicus to extract the DW width  $\xi_P$ ,

$$P_r(s) = P_r^\infty \tanh[(s - s_0)/\xi_P], \quad (1)$$

where  $P_r$  is the rotating component of the polarization,  $P_r^\infty$  is its asymptotic value far away from the domain wall,  $s$  is the coordinate perpendicular to the domain wall, and  $s_0$  is the position of the domain wall. In this section, different from below and the main article, polarization profiles are calculated from ionic positions and formal ionic charges (Bi<sup>3+</sup>, Fe<sup>3+</sup>, and O<sup>2-</sup>). Tests indicated that applying the more sophisticated Born effective charges changed the resulting polarization essentially only by a prefactor. The DW energies are close to those of Diéguez [7] and do not change very strongly with supercell size. Polarization and tilt profiles (Fig. 2) are also converged with respect to supercell size.

Figure 1 shows the layer-resolved ionic sublattice displacements compared to a paraelectric reference structure without octahedral tilts. The displacement profiles are atomically sharp.



| type | $n_{\text{atoms}}$ | $E$ (mJ/m <sup>2</sup> ) |                                       | $\xi_P$ (Å) | $\xi_A$ (Å) |
|------|--------------------|--------------------------|---------------------------------------|-------------|-------------|
|      |                    | this work                | Lit.                                  |             |             |
| 71°  | 80                 | 167                      | 152 <sup>a</sup> , 156 <sup>d</sup>   | 2.94±0.01   | 3.4±0.7     |
| 71°  | 100                | 170                      |                                       | 2.94±0.05   | 2.4±0.4     |
| 71°  | 120                | 172                      | 167 <sup>a</sup> , 143.2 <sup>c</sup> | 2.94±0.04   | 2.6±0.3     |
| 71°  | 160                |                          | 128 <sup>b</sup>                      |             |             |
| 109° | 80                 | 60                       | 62 <sup>a</sup> , 53 <sup>d</sup>     | 1.8±0.2     | 0.4         |
| 109° | 100                | 60                       |                                       | 2.0±0.1     | 0.4         |
| 109° | 120                | 63                       | 62 <sup>a</sup> , 52.9 <sup>c</sup>   | 1.9±0.1     | 0.1         |
| 109° | 160                |                          | 33 <sup>b</sup>                       |             |             |
| 180° | 80                 | 94                       | 74 <sup>a</sup> , 71 <sup>d</sup>     | 1.63±0.06   | –           |
| 180° | 100                | 86                       |                                       | 1.67±0.05   | –           |
| 180° | 120                | 84                       | 82 <sup>a</sup> , 81.9 <sup>c</sup>   | 1.67±0.04   | –           |
| 180° | 140                | 86                       |                                       | 1.67±0.04   | –           |
| 180° | 160                |                          | 98 <sup>b</sup>                       |             |             |

<sup>a</sup> Diéguez *et al.*[7], LDA+ $U$ ,  $U=4$  eV

<sup>b</sup> Wang *et al.*[6], GGA+ $U$ ,  $U=7$  eV,  $J=1$  eV

<sup>c</sup> Chen *et al.*[8], GGA+ $U$ ,  $U=3$  eV

<sup>d</sup> Ren *et al.*[9], LDA+ $U$ ,  $U=3.87$  eV

TABLE II. DW energies  $E$  and DW widths ( $\xi_P$ : polarization,  $\xi_A$ : tilt wall width) as function of the number of atoms  $n_{\text{atoms}}$  contained in the supercell. Errors are standard errors of the fit.

### Electronic potential step at the domain wall

Figure 3 depicts the magnitude of the electrostatic open-circuit potential step at the domain wall in the ground state (without excitons). These data are also listed in Table III. The

| $n_{\text{atoms}}$ | $-\Delta V_e^{\text{DW}}$ (mV) |       | $d_{\text{DW}}$ (Å) |      |
|--------------------|--------------------------------|-------|---------------------|------|
|                    | 71°                            | 109°  | 71°                 | 109° |
| 160                | 187                            | -18.3 | 22.1                | 31.2 |
| 200                | 159                            | -5.8  | 27.6                | 39.0 |
| 240                | 150                            | 2.9   | 33.2                | 46.8 |
| 280                | 157                            | 5.6   | 38.7                | 54.6 |
| ∞                  | 133                            | 17.3  | ∞                   | ∞    |

TABLE III. Electrostatic open-circuit potential step  $-\Delta V_e^{\text{DW}}$  of the 71° and 109° domain walls without excitons as a function of the domain-wall distance  $d_{\text{DW}}$  (the number of atoms in the supercell,  $n_{\text{atoms}}$ ), as depicted in Fig. 3.

potential converges to a positive number for both walls, so that it has the opposite sign compared to the polarization-based potential. We obtain the limit  $\Delta V_e^{\text{DW}}(\infty)$  of the potential step for large domain-wall distances  $d_{\text{DW}}$  by fitting with a power law:

$$\Delta V_e^{\text{DW}}(d_{\text{DW}}) = \Delta V_e^{\text{DW}}(\infty) + c \cdot d_{\text{DW}}^p, \quad (2)$$

where  $\Delta V_e^{\text{DW}}(\infty)$ ,  $c$ , and  $p$  are fit parameters. The resulting exponents are  $p_{71^\circ \text{ DW}} = -2.00$  and  $p_{109^\circ \text{ DW}} = -2.07$ .

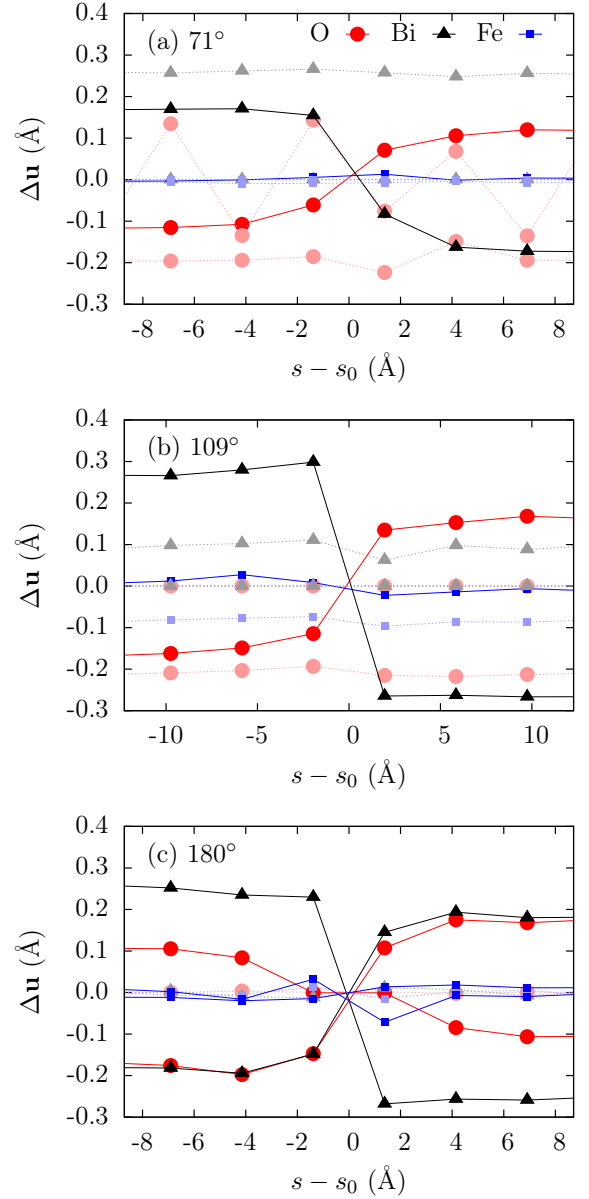

FIG. 1. The three cartesian components of the atomic displacements from the paraelectric, tilt-free phase in each atomic layer (a) for the 71° domain wall, (b) for the 109° domain wall, and (c) for the 180° domain wall in the coordinate system spanned by the supercell vectors: pseudocubic [110],  $\bar{1}\bar{1}0$ , and [001] directions (71° wall); [100], [011], and  $0\bar{1}1$  (109° wall);  $\bar{1}\bar{1}0$ , [110], and [001] (180° wall). Components that nominally remain constant across the domain wall are transparent.  $s_0$  is the position of the domain wall. The supercells contained 120 atoms.

### Calculation of the polarization-based potential

The ferroelectric polarization was calculated from ionic displacements from ideal perovskite positions using direction-averaged Born effective charges  $Z^*$  of the  $R3c$  phase ( $Z_{\text{Bi}}^* = 4.865$ ,  $Z_{\text{Fe}}^* = 3.886$ ,  $Z_{\text{O}}^* = -2.917$ ). First a smooth curve was fitted to the polarization profile perpendicular to the domain

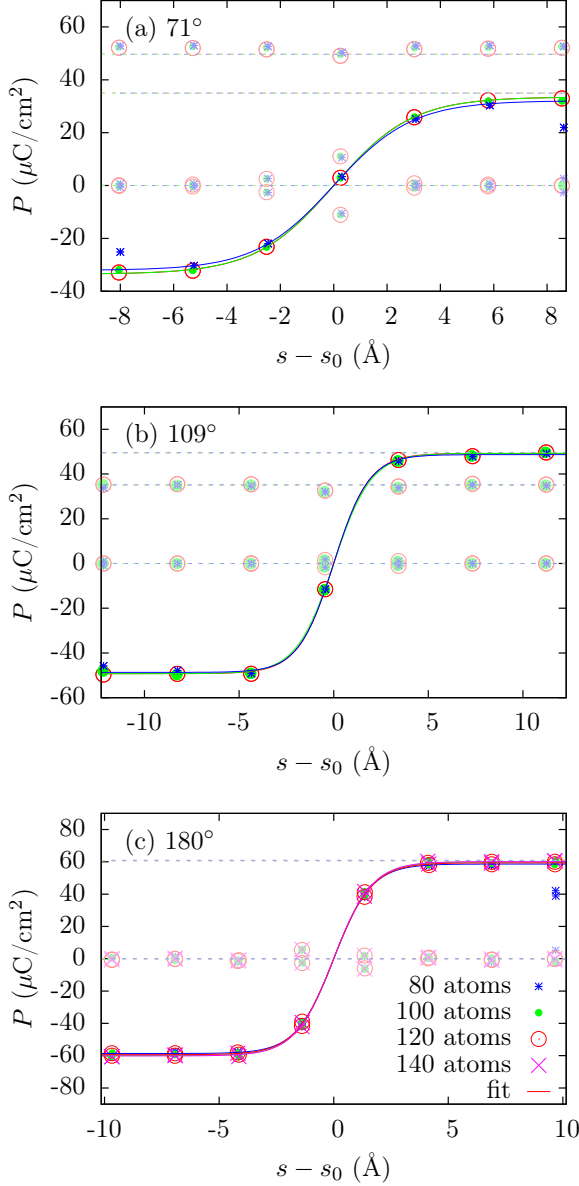

FIG. 2. Polarization  $P$  profiles for different supercell sizes (a) for the  $71^\circ$ , (b) for the  $109^\circ$  domain wall, and (c) for the  $180^\circ$  wall. Components that do not change sign at the domain wall are drawn transparent. Dashed transparent lines are the bulk reference. The profiles were fit according to Eq. (1).  $s_0$  is the position of the domain wall.

wall [ $P_s$  in Fig. 1 (c) and Fig. 2 (c) in the main article] using the program gnuplot. We employed a symmetric fit function of the form

$$P_s(s) = P_s^{(0)} - \frac{P_s^{(1)}}{\cosh^2\left(\frac{s-s_0}{\xi}\right)}, \quad (3)$$

where  $P_s^0$ ,  $P_s^1$ ,  $s_0$ , and  $\xi$  are fit parameters. The polarization-based electronic potential was then calculated as (compare

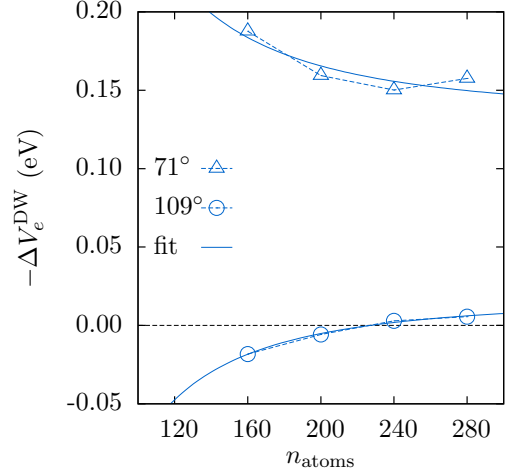

FIG. 3. Electrostatic potential step (electronic potential drop) at the  $71^\circ$  and the  $109^\circ$  domain wall without excitons as a function of the number of atoms  $n_{\text{atoms}}$  in the supercell (which is proportional to the domain-wall distance).

Eq. (8) in Ref. [10])

$$V_e^{\text{pb}}(s) = -\frac{1}{\epsilon_{ss}} \int_{s^-}^s (P_s(s') - P_s(s^-)) ds', \quad (4)$$

where  $s^-$  is a position in the domain interior on the left hand side of the domain wall, and  $\epsilon_{ss}$  is the calculated electronic dielectric constant for an electric field perpendicular to the domain-wall plane (see below). For  $P_s(s)$  we used the fitted curve from Eq. (3).

### Electronic and lattice screening

The screening (the real part of the static dielectric constant  $\epsilon$ ) is calculated *ab initio* using the primitive rhombohedral cell and a  $k$ -point mesh of  $10 \times 10 \times 10$  points.  $\epsilon$  is diagonal in the coordinate system spanned by the hexagonal lattice vectors (the pseudocubic  $[111]$ ,  $[\bar{1}10]$ , and  $[\bar{1}\bar{1}2]$  directions, parallel and perpendicular to the ferroelectric polarization). The electronic contribution  $\epsilon^e$  has the eigenvalues 7.4, 8.1, and 8.1, the lattice (ionic) contribution has the eigenvalues 21, 37, and 37. In order to obtain the screening in the direction  $s$  perpendicular to a domain wall, one needs to rotate  $\epsilon$  and obtains  $\epsilon_{ss}^e = 7.6$ ,  $\epsilon_{ss}^{\text{ion}} = 26$ , and  $\epsilon_{ss}^{\text{total}} = 34$  for the  $71^\circ$  domain wall and  $\epsilon_{ss}^e = 7.9$ ,  $\epsilon_{ss}^{\text{ion}} = 32$ , and  $\epsilon_{ss}^{\text{total}} = 40$  for the  $109^\circ$  domain wall. Both in the case of the polarization-based potential in the ground state and in the case of the photovoltage, screening is included *a posteriori*. For the polarization-based potential we use  $\epsilon_{ss}^{\text{total}}$ , for the photovoltages we use an effective dielectric constant  $\epsilon_{ss}^{\text{eff}}$  that replaces the electronic screening  $\epsilon_{ss}^e$  that is automatically included by the total (electronic and lattice)

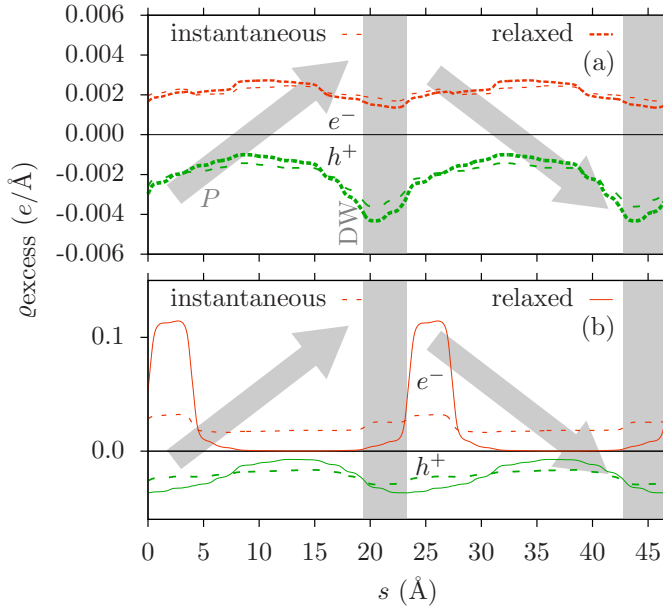

FIG. 4. Smoothed densities of excess electron and hole for excitons ( $X$ ) at the  $109^\circ$  domain wall before (“instantaneous”) and after (“relaxed”) polaron formation: (a) for an  $X$  density of  $0.1 X$  per 120-atom supercell (a planar  $X$  density of  $\approx 3.3 \cdot 10^{13} X/\text{cm}^2$ ) a large polaron forms, (b) for an  $X$  density of  $1 X$  per 120-atom supercell ( $\approx 3.3 \cdot 10^{14} X/\text{cm}^2$ ) a small polaron forms.

screening:

$$\epsilon_{ss}^{\text{eff}} = \frac{\epsilon_{ss}^{\text{ion}} + \epsilon_{ss}^e}{\epsilon_{ss}^e}. \quad (5)$$

The effective dielectric constant is  $\epsilon_{ss}^{\text{eff}} = 4.4$  for the  $71^\circ$  DW and  $\epsilon_{ss}^{\text{eff}} = 5.0$  for the  $109^\circ$  DW.

### Excitonic densities

Figure 4 shows the densities of excess electron and hole for an exciton at the  $109^\circ$  domain wall. Similar to the case of the  $71^\circ$  wall (see Fig. 3 in the main article), a large or small exciton polaron forms depending on the exciton density.

### Photovoltage

Figures 5 and 6 show all calculated photovoltage profiles for the  $71^\circ$  and the  $109^\circ$  domain wall in the 280-atom supercell.

The open-circuit (OC) voltage profiles were obtained from the short-circuit (SC) voltage profiles by adding a constant gradient such that in the domain interior the resulting OC voltage slope vanishes, as depicted in Fig. 7.

Table IV contains the calculated short-circuit and open-circuit domain-wall photovoltages obtained with different supercell sizes (different domain-wall distances), and those ex-

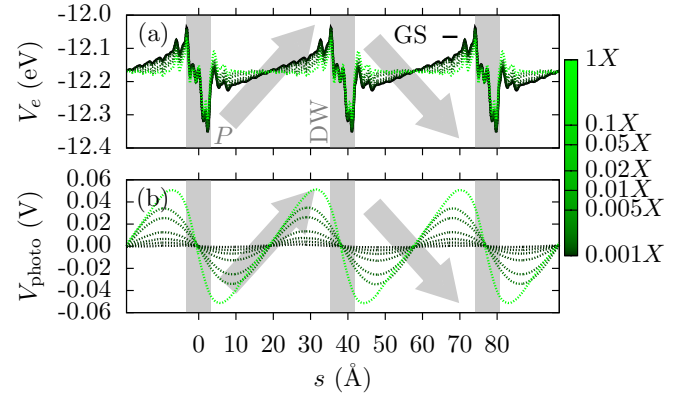

FIG. 5. (a) Ground-state and excited-state potential profile for exciton densities from 0.001 to 1 excitons ( $X$ ) per 280-atom supercell with  $71^\circ$  domain walls, (b) photovoltage profiles for these densities.

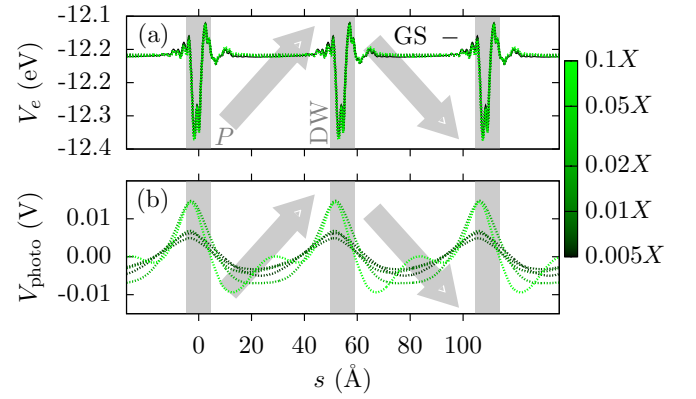

FIG. 6. The same as Fig. 5 for the  $109^\circ$  domain wall. Exciton densities range from  $0.005 X$  to  $0.1 X$  per supercell.

trapolated to the limit of infinitely large domain-wall distances. In the case of the  $71^\circ$  domain wall the extrapolated voltages (numbers in **boldface** in Tab. IV) are depicted in Fig. 7 in the main article. In the case of the  $109^\circ$  domain wall it is not possible to perform such an extrapolation because there is no strongly confining potential slope. Instead we depict the range of photovoltages between that of the largest supercell (280 atoms), and the largest photovoltage as a function of supercell size (numbers in **boldface** in Tab. IV).

### Parameters used in the rate equation

*Light penetration depth in a BiFeO<sub>3</sub> film* The penetration depth calculated from our first-principles absorption coefficient (which is similar to the one measured in Ref. 11) is about 33 nm at the photon energy of 3.06 eV that was used in experiment, such that about 95% of the penetrating light is absorbed in a 100 nm thick film. In Ref. 12 the penetration depth was estimated to be 50 nm, which would result in 86% of the penetrating light being absorbed.

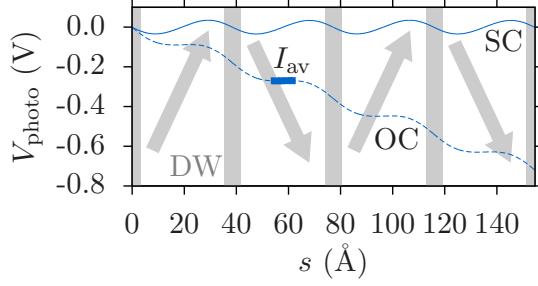

FIG. 7. Short-circuit (SC) photovoltage profile (thin solid line), open-circuit (OC) photovoltage profile (dashed line) for a 280-atom supercell with  $71^\circ$  domain walls, and the interval  $I_{av}$  (thick solid line) in which the average voltage slope was compensated by a constant gradient.

*Carrier diffusion length* It is difficult to accurately estimate the photocarrier diffusion length  $l_{diff}$ , therefore two different numbers are considered in the main article. An upper boundary should be the length of a ferroelectric domain.

*Exciton density at the domain wall* The planar exciton density  $n_X^{DW}$  is given by the number of excitons  $N_X$  and the domain-wall area  $A_{DW}$  contained in the supercell,  $n_X^{DW} = N_X / (2A_{DW})$ . The domain-wall area is  $A_{DW} \approx 42.7 \text{ \AA}^2$  for the  $71^\circ$  domain wall and  $A_{DW} \approx 30.2 \text{ \AA}^2$  for the  $109^\circ$  domain wall. Assuming that all photocarriers within  $l_{diff}$  reach the domain walls, the exciton density can be expressed as  $n_X = n_X^{DW} / l_{diff}$ , where  $n_X^{DW}$  is the planar exciton density at the domain wall. Then Eq. (3) in the main article becomes

$$I_{light} = \frac{n_X^{DW} E_{photon} d_{film}}{l_{diff}(1-R)\tau}. \quad (6)$$

#### Extrapolation of domain-wall photovoltages to large domain-wall distances

Figure 8 shows the open-circuit photovoltage as a function of the distance between two  $71^\circ$  domain walls  $d_{DW}$ . The photovoltage does not yet converge for our employed  $d_{DW}$  (supercells with up to 280 atoms), therefore we extrapolate it to the limit of large  $d_{DW}$  by means of a fit function:

$$V_{photo}^{DW}(d_{DW}) = V_{photo}^{DW}(\infty) - \Delta V_{photo}^{DW} e^{-b d_{DW}^{3/2}}, \quad (7)$$

where  $V_{photo}^{DW}(\infty)$ ,  $\Delta V_{photo}^{DW}$ , and  $b$  are fit parameters.  $V_{photo}^{DW}(\infty)$  is the extrapolated domain-wall photovoltage that is used in the main article. The fit function was chosen based on the exponential decay of the wave function of a particle in a linear potential (Airy function [13]). The data for the largest considered  $X$  density of 1  $X$  per supercell could not be extrapolated to large  $d_{DW}$  and were therefore left out of the analysis. In the case of the  $109^\circ$  domain wall, see Fig. 9, the domain-wall photovoltage increases, then decreases with increasing

| $n_X$ | $n_{atoms}$ | $71^\circ$ DW |           |             |              | $109^\circ$ DW |           |              |              |
|-------|-------------|---------------|-----------|-------------|--------------|----------------|-----------|--------------|--------------|
|       |             | $SC_{us}$     | $OC_{us}$ | OC          | $d_{DW}$ (Å) | $SC_{us}$      | $OC_{us}$ | OC           | $d_{DW}$ (Å) |
| 0.005 | 120         | 1.47          | 3.68      | 0.829       | 16.6         | 2.47           | -0.281    | -0.0558      | 23.4         |
|       | 160         |               |           |             | 22.1         |                |           |              | 31.2         |
|       | 200         | 3.86          | 11.0      | 2.48        | 27.6         | 5.77           | 12.4      | 2.46         | 39.0         |
|       | 240         | 5.76          | 15.1      | 3.40        | 33.2         | 6.47           | 15.7      | <b>3.12</b>  | 46.8         |
|       | 280         | 7.85          | 18.1      | 4.08        | 38.7         | 11.7           | 5.36      | <b>1.06</b>  | 54.6         |
|       | $\infty$    |               | 23.9      | <b>5.38</b> | $\infty$     |                |           |              | $\infty$     |
| 0.01  | 120         | 2.90          | 7.28      | 1.64        | 16.6         | 4.85           | 0.03      | 0.00596      | 23.4         |
|       | 160         | 4.03          | 10.3      | 2.32        | 22.1         |                |           |              | 31.2         |
|       | 200         | 7.16          | 20.4      | 4.60        | 27.6         | 10.9           | 21.0      | 4.17         | 39.0         |
|       | 240         | 10.8          | 29.1      | 6.56        | 33.2         | 14.2           | 26.0      | <b>5.17</b>  | 46.8         |
|       | 280         | 14.4          | 36.0      | 8.11        | 38.7         | 8.49           | 6.13      | <b>1.22</b>  | 54.6         |
|       | $\infty$    |               | 52.9      | <b>11.9</b> | $\infty$     |                |           |              | $\infty$     |
| 0.02  | 120         | 5.66          | 14.2      | 3.20        | 16.6         | 8.92           | -0.39     | -0.0775      | 23.4         |
|       | 160         |               |           |             | 22.1         |                |           |              | 31.2         |
|       | 200         | 13.3          | 37.5      | 8.45        | 27.6         | 17.6           | 35.4      | <b>7.03</b>  | 39.0         |
|       | 240         | 20.1          | 54.7      | 12.3        | 33.2         | 20.2           | 33.3      | 6.62         | 46.8         |
|       | 280         | 26.5          | 68.9      | 15.5        | 38.7         | 11.4           | 8.69      | <b>1.73</b>  | 54.6         |
|       | $\infty$    |               | 111       | <b>25.0</b> | $\infty$     |                |           |              | $\infty$     |
| 0.05  | 120         | 13.2          | 33.2      | 7.48        | 16.6         | 17.1           | 1.58      | 0.314        | 23.4         |
|       | 160         |               |           |             | 22.1         |                |           |              | 31.2         |
|       | 200         | 28.2          | 79.1      | 17.8        | 27.6         | 28.7           | 50.9      | 10.1         | 39.0         |
|       | 240         | 41.1          | 113       | 25.5        | 33.2         | 33.6           | 53.8      | <b>10.7</b>  | 46.8         |
|       | 280         | 52.0          | 138       | 31.1        | 38.7         | 22.7           | 3.95      | <b>0.785</b> | 54.6         |
|       | $\infty$    |               | 186       | <b>41.9</b> | $\infty$     |                |           |              | $\infty$     |
| 0.1   | 120         | 23.8          | 59.7      | 13.5        | 16.6         | 26.3           | -3.04     | 0.604        | 23.4         |
|       | 160         | 28.5          | 77.0      | 17.3        | 22.1         | 21.8           | 20.7      | 4.11         | 31.2         |
|       | 200         | 44.2          | 123       | 27.7        | 27.6         | 38.0           | 54.9      | <b>10.9</b>  | 39.0         |
|       | 240         | 59.4          | 162       | 36.5        | 33.2         | 38.2           | 35.4      | 7.03         | 46.8         |
|       | 280         | 69.3          | 180       | 40.6        | 38.7         | 24.2           | 23.4      | <b>4.65</b>  | 54.6         |
|       | $\infty$    |               | 193       | <b>43.5</b> | $\infty$     |                |           |              | $\infty$     |
| 1     | 120         | 83.8          | 165       | 37.2        | 16.6         |                |           |              | 23.4         |
|       | 160         | 83.8          | 173       | 39.0        | 22.1         |                |           |              | 31.2         |
|       | 200         | 90.9          | 175       | 39.4        | 27.6         |                |           |              | 39.0         |
|       | 240         | 98.1          | 189       | 42.6        | 33.2         |                |           |              | 46.8         |
|       | 280         | 102           | 172       | 38.8        | 38.7         |                |           |              | 54.6         |
|       | $\infty$    |               |           |             |              |                |           |              |              |

TABLE IV. Calculated short-circuit (SC) and open-circuit (OC) domain-wall photovoltages  $V_{photo}^{DW}$  for different domain-wall distances  $d_{DW}$  (different numbers of atoms  $n_{atoms}$  in the supercell) and extrapolations to infinitely large domain-wall distances as a function of the number of excitons  $n_X$  per supercell for the  $71^\circ$  and the  $109^\circ$  domain walls. Unscreened voltages are marked by the subscript “us”, such as  $SC_{us}$ . The photovoltages printed in **boldface** are the ones drawn in Fig. 7 in the main article.

domain-wall distance. Here we cannot easily extrapolate to large domain-wall distances, instead we consider the maximum photovoltage as a function of supercell size as an upper limit. As a lower limit we take the photovoltage of the largest considered domain-wall distance.

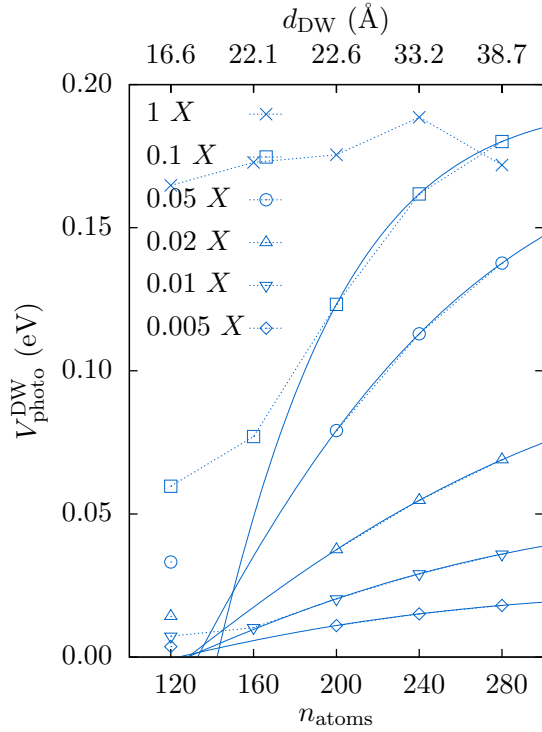

FIG. 8. Open-circuit photovoltage of the  $71^\circ$  domain wall as a function of the number of atoms  $n_{\text{atoms}}$  in the supercell and of the distance between domain walls,  $d_{\text{DW}}$  (data points from Table IV). Solid lines are fits with Eq. (7), dotted lines are a guide to the eye.

#### Extrapolation of domain-wall photovoltages to low light intensities

The photovoltages shown in Fig. 7 in the main article were extrapolated to low exciton densities (low light intensities  $I$ ) with a power law of the form

$$V_{\text{photo}}^{\text{DW}}(I) = V_{\text{photo}}^{\text{DW}}(I_0) \left( \frac{I}{I_0} \right)^p \quad (8)$$

that was optimized using the three data points corresponding to the lowest light intensities. In the case of the  $71^\circ$  domain wall  $p \approx 1.14$ . The photovoltage data of the  $109^\circ$  DW exhibit too much noise to safely extrapolate them to low light intensities.

#### Smoothing of charge densities and potential

The rapid and strong oscillations of charge densities and electronic potential at atomic nuclei, which obscure variations on a larger scale, were smoothed in the following way: First the charge density or potential was averaged in a plane parallel to the domain-wall plane [in the  $r$ - $t$  plane, compare Figs. 1(a) and 2(a) in the main article], then a sliding-window average over an  $s$  interval of one atomic plane spacing, like in Ref. [10], was applied to the excess charge carrier densities.

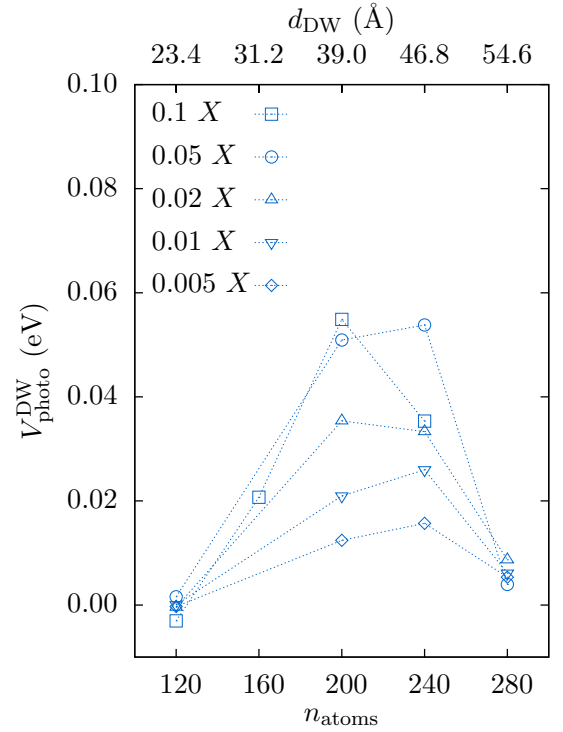

FIG. 9. The same as Fig. 8 for the  $109^\circ$  domain wall. Note the change of scale.

In order to smoothen the potential a low-pass filter was applied that removed wavelengths up to one atomic plane spacing. The two smoothening methods should be roughly equivalent, and it is only for historical reasons that one was used for the densities and the other for the potential.

---

\* skoerbel@uni-muenster.de

- [1] J. M. Moreau, C. Michel, R. Gerson, and W. J. James, “Ferroelectric  $\text{BiFeO}_3$  X-ray and neutron diffraction study,” *Journal of Physics and Chemistry of Solids* **32**, 1315 – 1320 (1971).
- [2] Andrzej Palewicz, R. Przeniosło, Izabela Sosnowska, and AW Hewat, “Atomic displacements in  $\text{BiFeO}_3$  as a function of temperature: neutron diffraction study,” *Acta Crystallographica Section B: Structural Science* **63**, 537–544 (2007).
- [3] A Palewicz, I Sosnowska, R Przenioslo, and AW Hewat, “ $\text{BiFeO}_3$  crystal structure at low temperatures,” *Acta Physica Polonica-Series A General Physics* **117**, 296 (2010).
- [4] P Fischer, M Polomska, I Sosnowska, and M Szymanski, “Temperature dependence of the crystal and magnetic structures of  $\text{BiFeO}_3$ ,” *Journal of Physics C: Solid State Physics* **13**, 1931 (1980).
- [5] Delphine Lebeugle, Dorothée Colson, A Forget, and Michel Viret, “Very large spontaneous electric polarization in  $\text{BiFeO}_3$  single crystals at room temperature and its evolution under cycling fields,” *Appl. Phys. Lett.* **91**, 022907 (2007).
- [6] Yi Wang, Chris Nelson, Alexander Melville, Benjamin Winchester, Shunli Shang, Zi-Kui Liu, Darrell G Schlom, Xiaoping Pan, and Long-Qing Chen, “ $\text{BiFeO}_3$  domain wall energies and

- structures: a combined experimental and density functional theory+U study,” *Phys. Rev. Lett.* **110**, 267601 (2013).
- [7] Oswaldo Diéguez, Pablo Aguado-Puente, Javier Junquera, and Jorge Íñiguez, “Domain walls in a perovskite oxide with two primary structural order parameters: First-principles study of  $\text{BiFeO}_3$ ,” *Phys. Rev. B* **87**, 024102 (2013).
- [8] Yun-Wen Chen, Jer-Lai Kuo, and Khian-Hooi Chew, “Polar ordering and structural distortion in electronic domain-wall properties of  $\text{BiFeO}_3$ ,” *J. Appl. Phys.* **122**, 075103 (2017).
- [9] Wei Ren, Yurong Yang, Oswaldo Diéguez, Jorge Íñiguez, Narayani Choudhury, and L. Bellaiche, “Ferroelectric Domains in Multiferroic  $\text{BiFeO}_3$  Films under Epitaxial Strains,” *Phys. Rev. Lett.* **110**, 187601 (2013).
- [10] B Meyer and David Vanderbilt, “Ab initio study of ferroelectric domain walls in  $\text{PbTiO}_3$ ,” *Phys. Rev. B* **65**, 104111 (2002).
- [11] V Železný, D Chvostová, L Pajasová, I Vrejoiu, and M Alexe, “Optical properties of epitaxial  $\text{BiFeO}_3$  thin films,” *Applied Physics A* **100**, 1217–1220 (2010).
- [12] Marin Alexe and Dietrich Hesse, “Tip-enhanced photovoltaic effects in bismuth ferrite,” *Nature Communications* **2**, 256 (2011).
- [13] Wolfgang P. Schleich, *Quantum Optics in Phase Space, Appendix E* (WILEY-VCH Verlag Berlin GmbH, 2001).
